# Supplementary material for: Funding the Frontier: Visualizing the Broad Impact of Science and Science Funding
Source: arXiv:2509.16323 source file (2025-09-19)
Supplement: Supplementary file 1 [file 10_SupplementalMaterial.tex]

\section{Supplemental Material}
\label{sec:09_Supplement} 

In this section, we introduce detailed information about dataset attributes, sub-datasets we use in the case study, and prediction models. 

% @xiaoyu: add data here
% 计算Case 1 and 2的amount (count number of rows)
% 不需要改下面的表格，直接在这里注释就行了，我会改表格的

% Top30 funder in case 2: 提供一个funder name list, ranked by funding amount and num_grant - 3列: funder_name, funding_amount, num_grant
% 再加两个数字：top 30 funder的grant涵盖了百分之多少的grant in all vis grants

\begin{table*}[!htbp]
\centering
\begin{tabular}{@{}lllp{8cm}p{3cm}} % Adjust the 6cm width as needed
\toprule
Entity Type & Dataset & Amount & Selected Meta Attributes & Field Attribute \\ \midrule
Grant & Dimensions & 7M & grant\_id, title, abstract, funding\_amount, funder\_org, research\_orgs, grant\_start\_date, grant\_end\_date, investigators & Fields of Research (ANZSRC 2020) \\
Paper & Dimensions, MAG & 140M & paper\_id, title, publication\_year, research\_orgs, investigators & \wyf{MAG field Level0-Level6} \\
Patent & Dimensions & 160M & patent\_id, title, filing\_year, assignee\_org & CPC category \\
Clinical Trial & Dimensions & 800K & clinical\_trial\_id, title, start\_year, end\_year, phase, \wyf{interventions} & mesh\_term \\
Policy & Overton & 10.9M & policy\_id, title, \wyf{policy\_source\_type} \& policy\_source\_title \& policy\_source\_country  (Org\_type (gov/IGO/think tank) & classifications \\
Newsfeed & Altmetric & 5.8M & newsfeed\_id, title, mention\_date, Outlet or Author, country & -- \\
Researcher & Dimensions & 51.7M & researcher\_id, name, gender (inferred), career\_age (inferred), research\_orgs &  \\
\bottomrule
\end{tabular}
\caption{xx}
\end{table*}

\begin{table}[]
\begin{tabular}{p{2cm}lll}
\toprule
Funding Impact Type & Linkage Type & Dataset & Amount \\ \midrule
Direct Outcome & grant-paper & Dimensions & 21M \\
Direct Outcome & grant-patent & Dimensions & 262K \\
Direct Outcome & grant-clinical trial & Dimensions & 28K \\
Broad Impact & paper-patent & Dimensions & 15M \\
Broad Impact & paper-clinical trial & Dimensions & 511K \\
Broad Impact & paper-policy & Overton & 13M \\
Broad Impact & paper-newsfeed & Altmetric & 6M \\
-- & paper-paper & Dimensions & 1.7B \\
-- & grant-PI & Dimensions & 9M \\
-- & paper-author & Dimensions & 461M \\ 
\bottomrule 
\end{tabular}
\caption{xxx}
\end{table}

% \begin{table}[ht]
% \centering
% \begin{tabular}{@{}lll@{}}
% \toprule
% Linkage Type & Dataset & Amount \\ \midrule
% grant-paper &  & 21M \\
% grant-patent &  & 262K \\
% grant-clinical trial &  & 28K \\
% paper-patent &  & 15M \\
% paper-clinical trial & \multirow{-5}{*}{Dimensions} & 511K \\
% paper-policy & Overton & 13M \\
% paper-newsfeed & Altmetric & 6M \\
% paper-paper &  & 1.7B \\
% grant-PI &  & 9M \\
% paper-author & \multirow{-3}{*}{Dimensions} & 461M \\ 
% \bottomrule
% \end{tabular}
% \caption{xxx}
% \end{table}

\wyf{TODO: add subsets in Two Cases}

% In support of transparent research practices and long-term open science goals, you are encouraged to make your supplemental materials available on a publicly-accessible repository.
% Please describe the available supplemental materials in the \hyperref[sec:supplemental_materials]{Supplemental Materials} section.
% These details could include (1) what materials are available, (2) where they are hosted, and (3) any necessary omissions. 

\begin{table}[ht]
\centering
\begin{tabular}{@{}lll@{}}
\toprule
& \multicolumn{2}{c}{Time difference ($Y$)} \\
Impact type & Case 1 & Case 2 \\
\midrule
direct\_paper & 5 & 3 \\
direct\_hit\_paper & 5 & 3 \\
direct\_disruptive\_paper &  5 & 3 \\
direct\_patent & 6 & 5 \\
direct\_clinical & 2 & - \\
broad\_patent & 9 & 8 \\
broad\_clinical & 8 & - \\
broad\_policy & 10 & 7 \\
broad\_newsfeed & 6 & 3 \\
\bottomrule
\end{tabular}
\caption{}
\label{tab:09_time_window_impact}
\end{table}

% \balance
